# Supplementary material for: Translating predictive distributions into informative priors
Source: arXiv:2303.08528 source file (2025-05-03)
Supplement: Supplementary file 1 [file pre-supplement.tex]

\usepackage{amsmath,amssymb,mathtools,bbm}
% I always seem to need tikz for something
\usepackage{tikz}
\usetikzlibrary{positioning, shapes, intersections, through, backgrounds, fit, decorations.pathmorphing}

\usepackage{algorithm}
\usepackage{algpseudocode}

\usepackage{setspace}
\onehalfspacing

\usepackage{lineno}
% \linenumbers

% \usepackage{xr}
% \makeatletter
% \newcommand*{\addFileDependency}[1]{% argument=file name and extension
%   \typeout{(#1)}
%   \@addtofilelist{#1}
%   \IfFileExists{#1}{}{\typeout{No file #1.}}
% }
% \makeatother

% \newcommand*{\myexternaldocument}[1]{%
%     \externaldocument{#1}%
%     \addFileDependency{#1.tex}%
%     \addFileDependency{#1.aux}%
% }

% \myexternaldocument{priors-by-optimisation}

% required for landscape pages. beware, they make build times very long.
\usepackage{pdflscape}
\usepackage{placeins}

% table - `gt' package uses these, often unimportant
%\usepackage{longtable}
\usepackage{booktabs}
\usepackage{colortbl}

\usepackage{color}
\definecolor{myredhighlight}{RGB}{180, 15, 32}
\definecolor{mydarkblue}{RGB}{0, 33, 79}
\definecolor{mymidblue}{RGB}{44, 127, 184}
\definecolor{mylightblue}{RGB}{166, 233, 255}
\definecolor{mywhwlow}{RGB}{234, 164, 99}

\usepackage{accents}
\newlength{\dhatheight}

\setcounter{secnumdepth}{3}

% \renewcommand{\floatpagefraction}{0.8}
% \renewcommand{\topfraction}{0.8}
% \renewcommand{\bottomfraction}{0.8}
% \renewcommand{\textfraction}{0.25}

% pd stands for: probability distribution and is useful to distringuish
% marignals for probabilities specifically p(p_{1}) and the like.

% pbbo stuff

% melding

% the q(x)w(x), "weighted target" density 
% for the moment I'm going to call it s(x), as that is the next letter of the 
% alphabet. Can change it later

% direct density estimate - replaces lambda.

% target weighting function

% constants - usually sizes of things

% locales - could switch to x and x'

% sugiyama stuff

% indices 

\DeclarePairedDelimiterX{\infdivx}[2]{(}{)}{%
  #1\;\delimsize\|\;#2%
}

\algrenewcommand\alglinenumber[1]{
    {\sf\footnotesize\color{lightgray}#1}}
\algrenewcommand\algorithmicrequire{\textbf{Inputs:}}
\algrenewcommand\algorithmicensure{\textbf{Postcondition:}}

\def\dodoi#1{doi: \href{https://doi.org/#1}{\nolinkurl{#1}}}
\def\dourl#1{\href{http://#1}{\nolinkurl{#1}}}
